# Supplementary material for: Automating Urban Soundscape Enhancements with AI: In-situ Assessment of Quality and Restorativeness in Traffic-Exposed Residential Areas
Source: arXiv:2407.05744 source file (2024-10-09)
Supplement: Supplementary file 2 [file appendix-start.tex]

\setcounter{section}{0}

\setcounter{table}{0}

\setcounter{figure}{0}
