# Supplementary material for: Automating Urban Soundscape Enhancements with AI: In-situ Assessment of Quality and Restorativeness in Traffic-Exposed Residential Areas
Source: arXiv:2407.05744 source file (2024-10-09)
Supplement: Supplementary file 3 [file next-appendix.tex]

\setcounter{table}{1}
